# Supplementary material for: Towards Anomaly Detection in Dashcam Videos
Source: arXiv:2004.05261 source file (2020-05-12)
Supplement: Supplementary file 1 [file appendix.tex]

% \appendixpage
% \section*{Appendix}

% \renewcommand{\the}{A-\arabic{equation}}
% % redefine the command that creates the equation no.
% \setcounter{equation}{0}  % reset counter 
\section*{APPENDIX}  % use *-form to suppress numbering
\label{sec:appendix}
\section{Implementation details of Optical Flow}
\label{sec:opt-flow}
For Optical Flow, the videos are sampled at a frame rate of 25 fps. We use the TV-L1 Optical Flow implementation available in OpenCV. We truncate the values to a range of $[-20, 20]$ and then re-scale the horizontal and vertical components of flow to a range of $[0, 255]$. We store optical flow for each video as JPEG files. This saves us from the computational expense of optical flow at training time. In our experiments, the optical flow is computed between two consecutive frames and it is normalized to a range of $[-1, 1]$ before being fed to the neural network. This strategy is the same as followed in \cite{simonyan2014two}.

\input{tables/architecture.tex}
